# Supplementary material for: Batch Distillation Data for Developing Machine Learning Anomaly Detection Methods
Source: arXiv:2510.18075 ancillary file (2026-04-10)
Supplement: Supplementary file 1 [file SI.pdf]

# Supporting Information for Batch Distillation Data for Developing Machine Learning Anomaly Detection Methods

Justus Arweiler,† Indra Jungjohann,† Aparna Muraleedharan,‡ Heike Leitte,¶ Jakob Burger,‡ Kerstin Münnemann,† Fabian Jirasek,*,† and Hans Hasse†

†*Laboratory of Engineering Thermodynamics, RPTU Kaiserslautern, Erwin-Schrödinger-Straße 44, 67663 Kaiserslautern, Germany*

‡*Technical University of Munich, Campus Straubing for Biotechnology and Sustainability, Laboratory for Chemical Process Engineering, Uferstraße 53, 94315 Straubing, Germany*

¶*Department of Computer Science, RPTU Kaiserslautern, Erwin-Schrödinger-Straße 44, 67663 Kaiserslautern, Germany*

E-mail: fabian.jirasek@rptu.de

## 1 Additional Information on the Batch Distillation Plant

### 1.1 Overview

The mapping of the labels in the P&I flowsheet shown in Figure 1 of the main paper to the corresponding parts of the plant is given in Table 1.

**Table 1:** Mapping of the labels in the P&I flowsheet shown in Figure 1 of the main paper to the corresponding parts of the plant.

| Label | Type | Description |
|---|---|---|
| Actuator | AV8 | Automatic valve for pressure control |
| | AV201 | Automatic valve for inline sampling line |
| | AV205 | Automatic valve for stopped-flow inline sampling |
| | AV709 | Automatic valve for nitrogen supply |
| | AV716 | Automatic valve for cooling water supply |
| | CHV1 | Check valve after reflux pump P701 |
| | CHV2 | Check valve after distillate pump P702 |
| | H001 | Heating tape |
| | H002 | Heating rod |
| | H701 | Heating element |
| | H702 | Heating element |
| | H704 | Heating element |
| | H706 | Heating element |
| | H708 | Heating element |
| | HV001 | Side-draw valve between V001 and C001 |
| | HV002 | Side-draw valve between C001 and C002 |
| | HV003 | Side-draw valve between C002 and C003 |
| | HV004 | Manual valve for sample specimen drawing |
| | HV005 | Manual valve for connection of inline sampling line to distillate buffer |
| | HV006 | Manual valve for product drain from V003 |
| | HV007 | Manual valve for ventilation to atmosphere |
| | HV008 | Manual valve for liquid drain in HE004 |
| | HV009 | Manual valve for offline sampling in V001 |
| | HV101 | Manual valve for nitrogen supply of PDI702 |
| | HV102 | Manual valve for nitrogen supply of PDI701 |
| | HV103 | Manual valve, nitrogen pressure regulator |
| | HV202 | Manual valve for closing inline sampling line |
| | M001 | Magnetic stirrer in V001 |
| | M701 | Motor unit for lifting table |
| | MSC701 | Motor unit for M001 |
| | P201 | Inline sampling pump |
| | P301 | Vacuum pump |
| | P701 | Reflux pump |
| | P702 | Distillate pump |
| | PRV001 | Pressure relief valve at G001 |
| | PRV201 | Pressure relief valve in front of QR201 |
| | TCU1 | Circulating thermostat for HE001, HE002, HE003 |
| | TCU2 | Circulating thermostat for HE004 |
| | TV1 | Throttle valve for pressure control |
| Equipment | C001 | Column section with structured laboratory packing |

**Table 1:** Continued.

| Label | Type | Parts of the plant |
|---|---|---|
| | C002 | Column section with structured laboratory packing |
| | C003 | Column section with structured laboratory packing |
| | F201 | Filter unit in inline sampling line |
| | G001 | Glass unit with multiple ports |
| | G002 | Glass unit with multiple ports |
| | HE001 | Glass condenser unit with spiral coil and multiple ports |
| | V001 | Reboiler vessel |
| | V002 | Buffer vessel |
| | V003 | Distillate receiver |
| | V201 | Pressure relief collection vessel |
| Sensor | CAM001 | Camera at HE001 |
| | CAM002 | Camera at V002 |
| | CAM003 | Camera at V003 |
| | FT201 | Mass flux sensor |
| | FT703 | Mass flux sensor |
| | FT704 | Mass flux sensor |
| | FYI702 | Flux sensor |
| | HE002 | Glass subcooling unit with spiral coil |
| | HE003 | Pre-heating unit, spiral coil above column |
| | HE004 | Condensation trap |
| | LS701 | Level sensor |
| | LS702 | Level sensor |
| | PI2 | Pressure indicator(difference to ambient pressure) |
| | PI8 | Pressure indicator for nitrogen supply |
| | PI201 | Pressure indicator in front of QR201 |
| | PDI701 | Differential pressure sensor |
| | PDI702 | Differential pressure sensor |
| | PY23 | Pressure sensor |
| | QR201 | Concentration measurement system, benchtop NMR unit |
| | SD001 | Microphone at reflux and distillate pump |
| | T001 | Temperature sensor |
| | T002 | Temperature sensor |
| | T701 | Temperature sensor |
| | T702 | Temperature sensor |
| | T703 | Temperature sensor |
| | T704 | Temperature sensor |
| | T705 | Temperature sensor |
| | T706 | Temperature sensor |
| | T708 | Temperature sensor |
| | T709 | Temperature sensor |
| | T711 | Temperature sensor |

**Table 1:** Continued.

| Label | Type | Parts of the plant |
|---|---|---|
| | T712 | Temperature sensor |

Information on the suppliers of the parts of the plant is given in Table 2.

**Table 2:** Suppliers of main components of the plant. Product labels are reported as available.

| Label | Supplier | Product label |
|---|---|---|
| AV201, AV205 | Rheodyne (IDEX Health & Science ) | MX, 2-position 6-port |
| AV8 | Bürkert Fluid Control Systems | Typ 2821 |
| AV709 | | Typ 6013 |
| AV716 | Gemü | Typ 102 |
| C001, C002, C003 | Iludest Destillationsanlagen | LM 2/S |
| V001, V002, V003 | | |
| FT201 | Bronkhorst | miniCoriFlow M12 |
| FT703, FT704 | | miniCoriFlow M14-ABD-330-S |
| FYI702 | Gems | Rotorflow RFO |
| H001 | Julabo | LC4 |
| H002 | HS-Heizelemente | Heating cartridge with Pt100 |
| H701 | SAF Wärmetechnik | |
| H702 | | |
| H704, H706, H708 | | |
| LS701, LS702 | Omron | E3H2-DS30B4M-M1 |
| P201 | FLUSYS | WADose Lite HP |
| P301 | Vacuubrand | MD 4C NT |
| P701 | Verder | VGS015 |
| P702 | | VGS015 |
| PDI701, PDI702 | BD sensors | DMD 831 |
| PY23 | MKS | Baratron 600 |
| QR201 | Magritek | Spinsolve 80 ULTRA Carbon |
| TCU1 | Julabo | HE-4 |
| TCU2 | Huber | TC-45 |

## 1.2 Safety Measures

To ensure the operational safety of the batch distillation process, several measures were implemented. The laboratory-scale distillation plant was placed in a fume hood and set on a drip pan to prevent contamination of the laboratory in the event of a leak. The pressure relief valve PRV1 was filled with paraffin oil to ensure a tight seal against ambient air inflow

when operating the batch distillation plant under vacuum conditions.

Several safety shut-down measures were implemented. All heating elements are shut down if either the level sensor LS701 in the reboiler vessel V001 signals "dry" for more than 10 seconds, or if the flow of cooling water FYI702 drops below a pre-defined threshold for more than 10 seconds, or if the pressure difference between the bottom and top of the columns section exceeds a pre-defined threshold. Furthermore, all heating elements shut down if the temperature of any heating element exceeds the lowest ignition point of any component in the feed mixture of the respective experiment. The plant is secured against accidental switch-on after a power loss and shuts down if connection to the process control system is lost for more than 30 seconds.

## 1.3 Ambient Data

Prior to each experimental run, the ambient conditions were measured (pressure, temperature, and humidity in the laboratory, and, additionally, the outside temperature). The ambient pressure was measured with a mercury barometer (Lambrecht meteo GmbH); pressure readings were corrected for altitude, temperature, capillary, and latitude according to [1]. For measuring ambient humidity and temperature, a Testo 635-1 temperature and humidity measuring instrument (Testo Ltd) was used. Humidity was measured with an accuracy of 2% of the reading, and temperature with ±0.3 K. For the outside temperature, the value from the Deutsche Wetterdienst in Kaiserslautern was used.

## 1.4 Calibration of Sensors

### Mass flux Sensors

The sensors FL703 and FL704, which measure the mass flow of the withdrawn product and the reflux, were calibrated by the manufacturer using a calibration-by-comparison method traceable to national standards of the Dutch Metrology Institute VSL.

### Pressure Sensors

The sensor PIC23, which measures the absolute pressure in the batch distillation plant, was calibrated by the manufacturer in accordance with ISO/IEC 17025 using a Fluke forced-piston gauge transfer standard, identification number 000210609, traceable to the United States National Institute of Standards and Technology (NIST). The differential pressure sensors PD701 and PD702 were calibrated by the manufacturer; the authors could obtain no further information.

### Temperature Sensors

The temperature sensors monitoring the temperatures inside the plant, TICS703, TICS705, TIS709, TIS711, and TIS712, were calibrated with a reference temperature calibration using an Isotech MicroK-100 Thermometry Bridge (Isothermal Technology Limited) combined with a Rosemount 162CE Long-Stem Standard Platinum resistance thermometer (Emerson Electric Company). The temperature sensors TICS701, TICS702, TICS704, TICS706, TICS708, TICS001, and TIS002 embedded in the plant's heating elements were calibrated by the manufacturers. We did not receive any related documents and therefore assume the standard measurement uncertainty of the used Pt100 temperature classes.

## 1.5 Offline Gas Chromatography

For offline measurement of mixture compositions in the plant, samples were drawn from V001 and V002 every 15 to 25 minutes, depending on the operating point of the experiment. First, the sample line was rinsed by drawing 1 ml of sample through it. Then, at least 0.5 ml of the sample was drawn. The mass of the samples was measured and recorded. Each sample was prepared with the internal standard 1,4-dioxane at a 4:1 mass ratio and analyzed on a gas chromatograph (GC) (Agilent 7890A). For the system (acetone + 1-butanol + methanol), as well as for the system (ethanol + 2-propanol), an Agilent Rtx-Wax column with a length

of 30 meters, an inner diameter of 320 µm, and a 1 µm film thickness was used with a flame ionization detector. For the analysis of the system (1-butanol + 2-propanol + water), an Agilent HP-InnoWax column with a length of 30 meters, an inner diameter of 320 µm, and 0.5 µm film thickness was used in combination with a thermal conductivity detector.

The GC analysis was calibrated using samples with known mass ratios and the same internal standard, 1,4-dioxane. For the system (1-butanol + 2-propanol + water), 10 samples, for the system (acetone + 1-butanol + methanol), 11 samples, and for the system (ethanol + 2-propanol), 9 samples were used.

## 1.6 Online NMR Spectroscopy

Online concentration measurements were performed using a Spinsolve 80 ULTRA Carbon benchtop NMR spectrometer (Magritek, QR201). A glass flow cell supplied by Magritek was positioned in the magnet bore; it consisted of a 1 mm inner-diameter capillary that expanded to 4 mm at the measuring coil. The spectrometer was initially shimmed with a reference sample of 95% $D_2O$ / 5% $H_2O$, yielding a signal-to-noise ratio of 50250 and a 0.34 Hz linewidth at 50% height. Before each experiment, a first- and second-order "quickshim" was performed while the process mixture was circulated through the cell at 0.2 ml min$^{-1}$. During operation, single-scan $^1$H NMR spectra were acquired every minute with a 90° flip angle and an acquisition time of 3.2 s. Spectra were processed using the Python library NMRglue[2]. An exponential line broadening of 1 Hz and zero-filling by a factor of 8 were applied, followed by automatic baseline correction using the adaptive penalized least-squares algorithm implemented in pybaselines[3–5]. Voigt profiles were then fitted to individual peaks with DEEP picker[6], providing peak positions, areas, and confidence values. To avoid errors from overlapping peaks, only distinct, non-overlapping spectral regions were used for each mixture.

Because internal standards cannot be added during dynamic operation, the first peak in the spectrum was fixed to a reference chemical shift. The mole fraction $x_i$ of compound $i$ was

determined from the summed areas $A_i$ of its multiplets via

$$x_i = \frac{\frac{A_i}{N_{\mathrm{H},i}}}{\sum_{i=0}^{N_{\mathrm{Mix}}} \frac{A_i}{N_{\mathrm{H},i}}} \tag{1}$$

where $N_{\mathrm{H},i}$ is the number of contributing protons in compound $i$ and $N_{\mathrm{Mix}}$ the number of components.

NMR spectra were collected once per minute, whereas plant sensor data were logged every second; thus, missing values were linearly interpolated. As NMR measurements are limited by flow-induced line broadening[7], the sampling pump P201 operated at 0.2 ml $\mathrm{min}^{-1}$, resulting in a measurable delay between sampling and spectrum acquisition. This delay $t_{\text{NMR-delay}}$ was determined from the known tubing volume and instantaneous pump rate $\dot{V}$:

$$t_{\text{NMR-delay}} = \frac{\sum \dot{V}_{\mathrm{P201}}}{V_{\text{Sample position-QR201}}} \tag{2}$$

The final database maps each spectrum to the corresponding sampling time in the distillation process. Peak assignments for the studied mixtures are shown in Figures 1-3, together with information on the peaks that were used for the quantitative evaluation.

The NMR magnet was thermostated at 26.5 °C. Since active cooling was unavailable, online monitoring had to be suspended during periods of elevated ambient temperature.

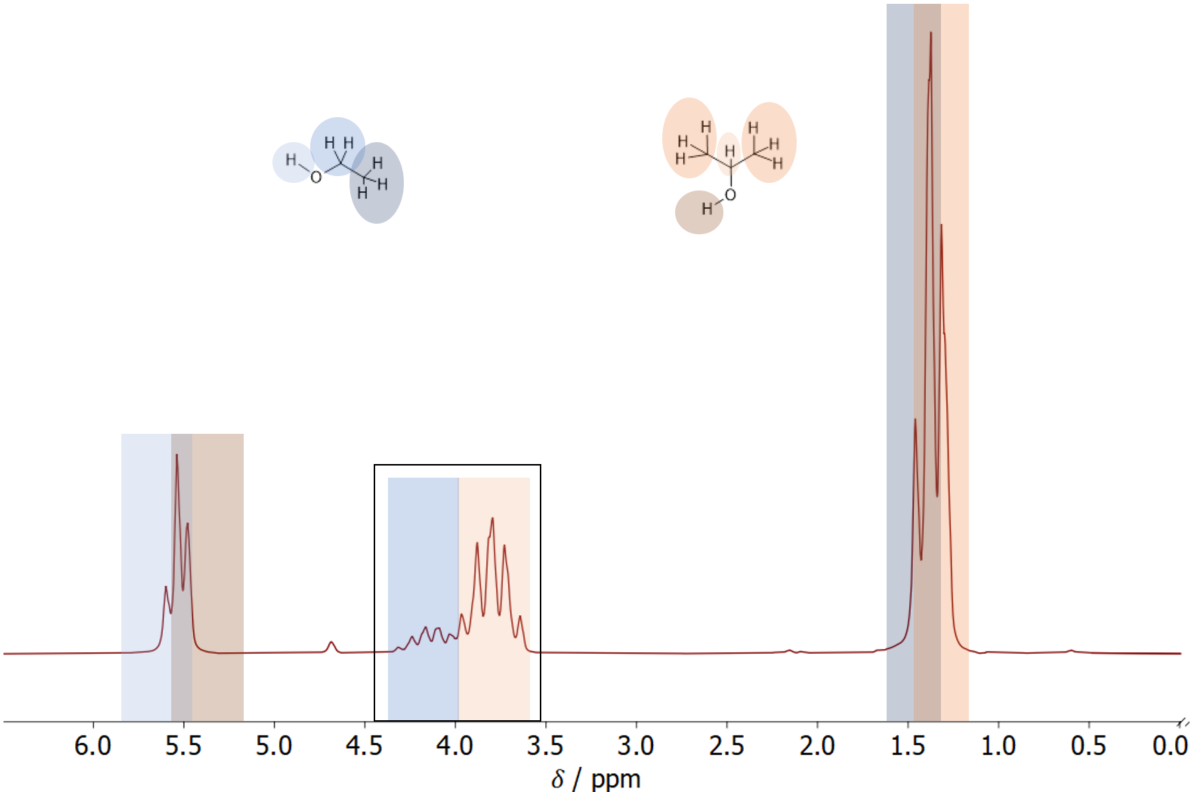


**Figure 1:** $^{1}$H NMR spectrum of a mixture containing (ethanol + 2-propanol). The black box marks the spectral region used for quantitative analysis.

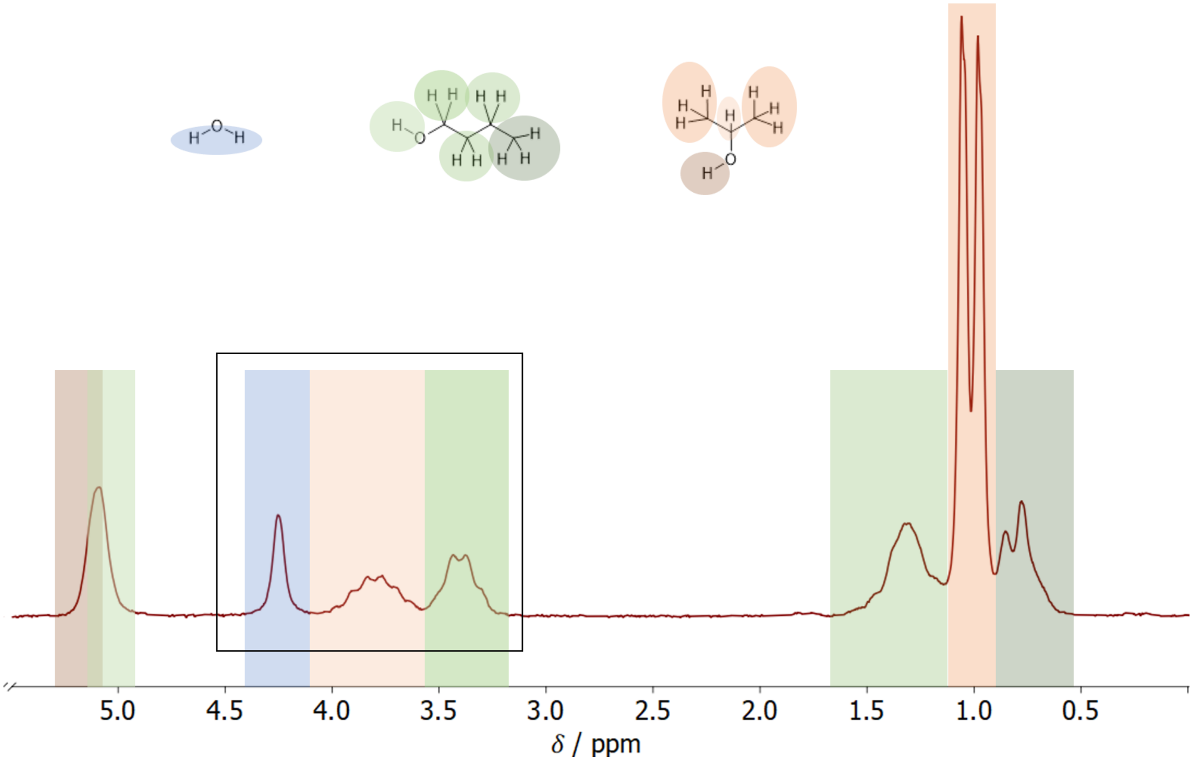


**Figure 2:** [1]H NMR spectrum of a mixture containing (1-butanol + 2-propanol + water). The black box marks the spectral region used for quantitative analysis.

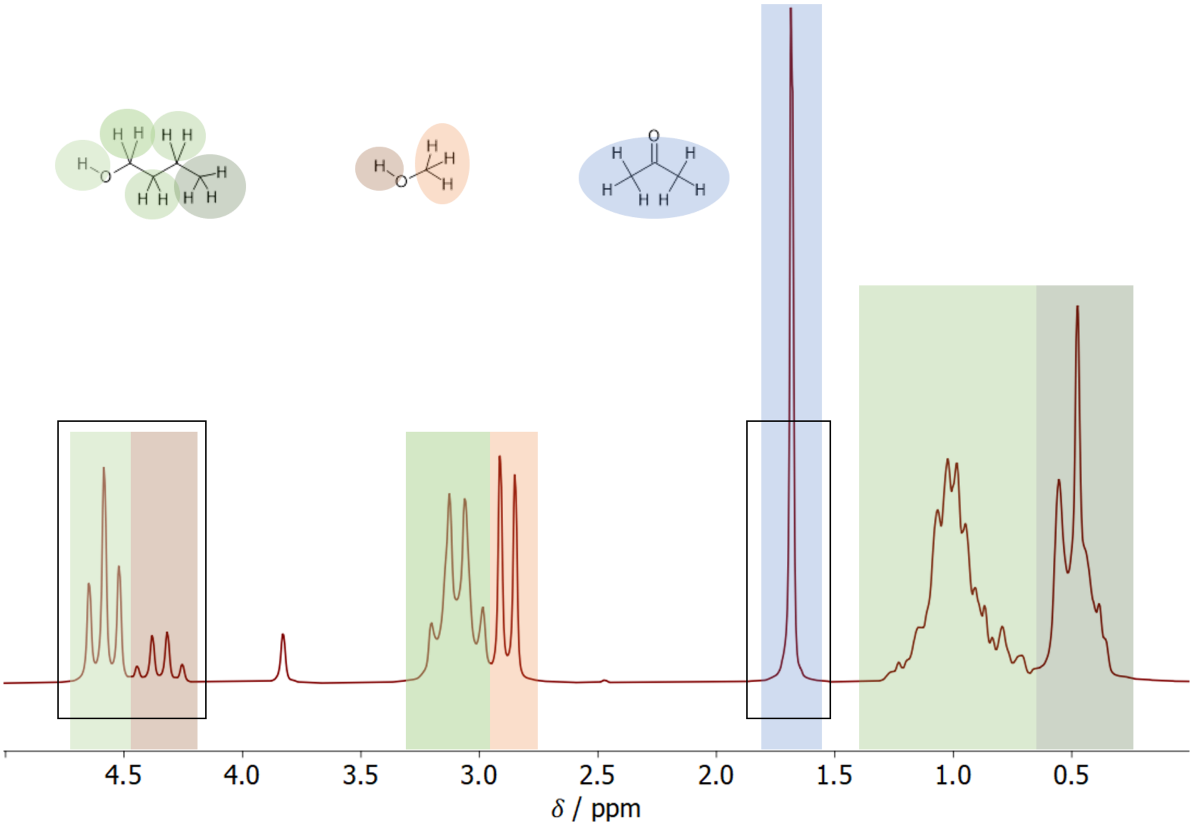


**Figure 3:** [1]H NMR spectrum of a mixture containing (acetone + 1-butanol + methanol). The black box marks the spectral region used for quantitative analysis.

## 2 Additional Information on the Mixtures

In Table 3, the chemicals and their manufacturers and purities are given. In the database, for each experiment, the analysis certificates of the used chemicals are provided along with the mixture information, if available. In Figures 4 and 5, the residue curves (at 1 bar) of the ternary mixtures used in this work, calculated using extended Raoult's Law with activity coefficients estimated using the NRTL model[8], are given. Both systems (acetone + 1-butanol + methanol) and (1-butanol + 2-propanol + water) show binary azeotropes, as indicated in the figures. Moreover, the system (1-butanol + 2-propanol + water) exhibits a liquid-liquid equilibrium (LLE). Most experiments in the database for this system used feed mixtures that avoid process conditions leading to LLE in the plant. Binary interaction parameters $\tau_{ij}$ of NRTL were fitted using isobaric experimental binary data at 1 bar from the Dortmund

Data Bank (DDB)[9]. The parameters are given in Table 4.

**Table 3:** Purities and manufacturers of components used in experimental campaigns in the batch distillation plant. Purity is reported as specified by the supplier's certificates of analysis.

| Component | Supplier | Lot-no. | Molar purity |
|---|---|---|---|
| Acetone | Supelco | I1324114 | 99.9% |
| 1-Butanol | Fisher Thermo Scientific | A0444653 | 99.9% |
| Ethanol | Sigma-Aldrich | STBK7309 | ≥ 99.9% |
| Methanol | Sigma-Aldrich | STBL4182 | 99.9% |
| 2-Propanol | Honeywell | M2360 | 99.99% |

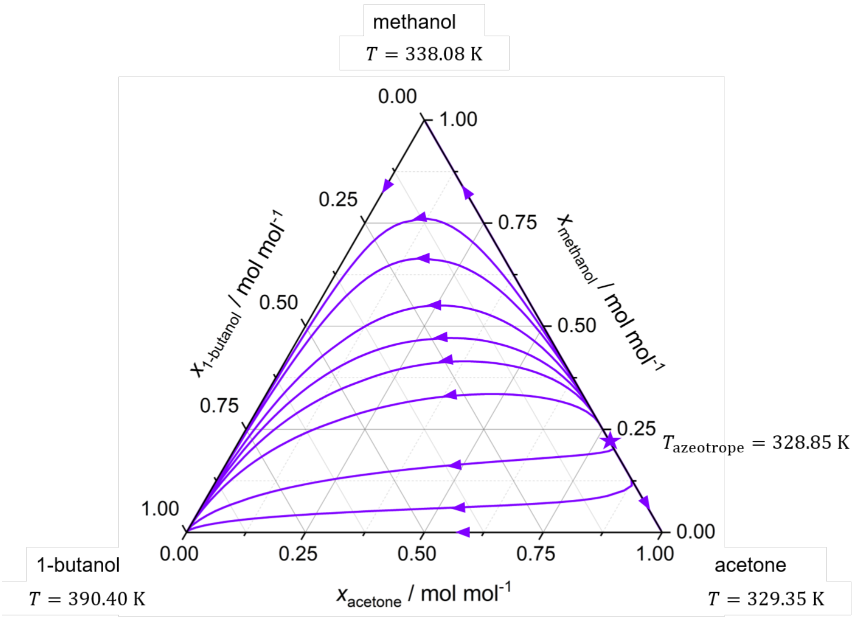


**Figure 4:** Residue curves for the system (acetone + 1-butanol + methanol) at 1 bar. Azeotropes are indicated with a star symbol. Boiling temperatures of the pure components and the azeotropic mixtures at 1 bar are specified.

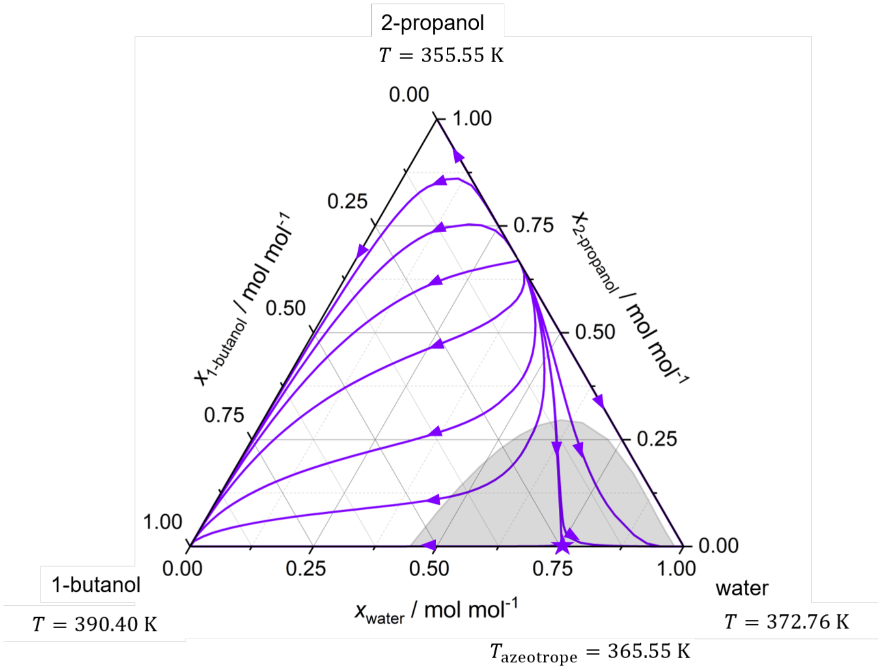


**Figure 5:** Residue curves for the system (1-butanol + 2-propanol + water) at 1 bar. Azeotropes are indicated with a star symbol. Boiling temperatures of the pure components and the azeotropic mixtures at 1 bar are specified.

**Table 4:** Interaction parameters $\tau_{ij}$ of the NRTL model[8] fitted to experimental data for the binary systems from the DDB[9].

| Component $i$ | Component $j$ | $\tau_{ij}$ | $\tau_{ji}$ |
|---|---|---|---|
| Acetone | 1-Butanol | 0.69823 | -0.06839 |
| Acetone | Methanol | 0.29423 | 0.33341 |
| 1-Butanol | 2-Propanol | -0.41247 | 0.46349 |
| 1-Butanol | Methanol | 0.63230 | -0.46038 |
| 1-Butanol | Water | 0.05864 | 3.75741 |
| Ethanol | 2-Propanol | 0.48856 | -0.45323 |
| 2-Propanol | Water | -0.10456 | 2.74607 |

# 3 Overview of the Experimental Dataset

In Figure 6, the availability of each data mode is depicted for each experiment in the database.

Table 5 gives an overview over the settings used for each operating point in the database.

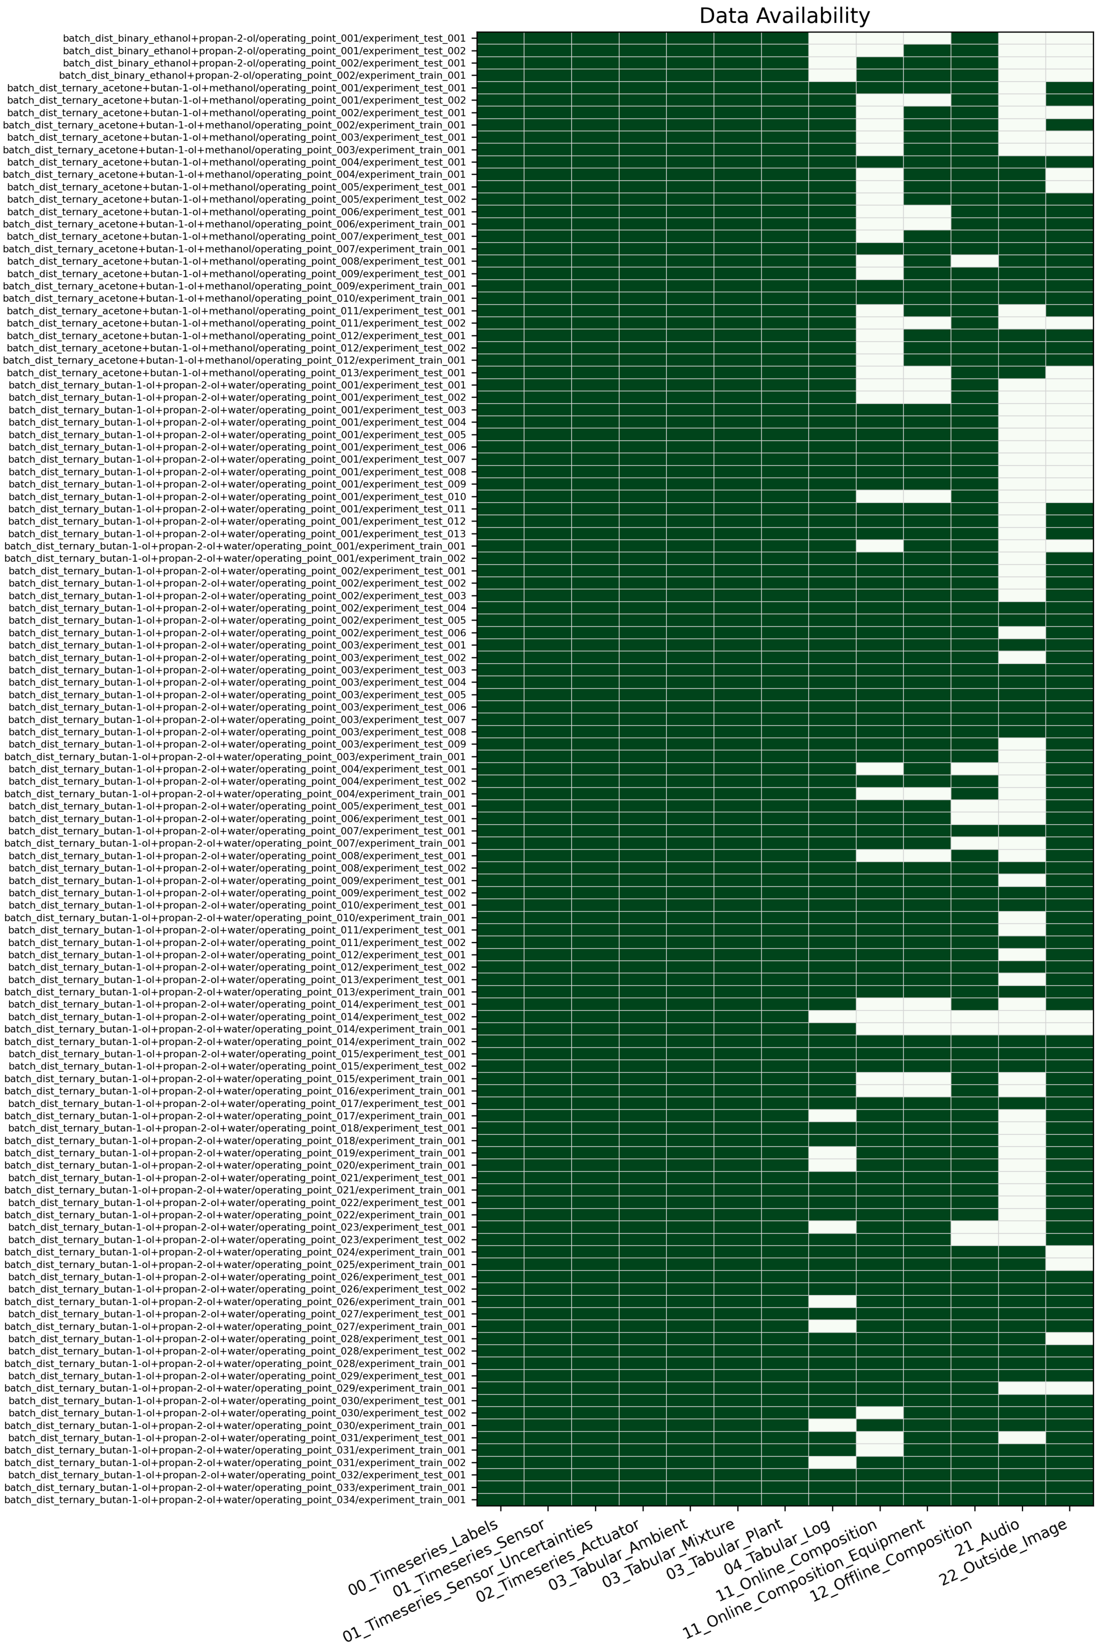


**Figure 6:** Availability of data modes for each experiment in the database. Green tiles mark available data modes, white tiles mark missing data.

**Table 5:** Operating points of experiments in the database and number of anomalies observed for each operating point. The order of components in the initial molar mixture composition column is the same as the order of components in the file name.

| ID | Initial molar mixture composition | $R$ / - | $p$ / mbar | $\dot{Q}$ / W | No. of anomalies |
|---|---|---|---|---|---|
| batch_dist_binary_ethanol+propan-2-ol/operating_point_001 | 0.7/0.3 | 0.2 | 300 | 175 | 7 |
| batch_dist_binary_ethanol+propan-2-ol/operating_point_002 | 0.7/0.3 | 1.33 | 300 | 175 | 3 |
| batch_dist_ternary_acetone+butan-1-ol+methanol/operating_point_001 | 0.33/0.33/0.33 | 2 | 650 | 175 | 2 |
| batch_dist_ternary_acetone+butan-1-ol+methanol/operating_point_002 | 0.33/0.33/0.33 | 1 | 550 | 140 | 1 |
| batch_dist_ternary_acetone+butan-1-ol+methanol/operating_point_003 | 0.33/0.33/0.33 | 0.66 | 300 | 157.5 | 1 |
| batch_dist_ternary_acetone+butan-1-ol+methanol/operating_point_004 | 0.33/0.33/0.33 | 6 | 350 | 175 | 1 |
| batch_dist_ternary_acetone+butan-1-ol+methanol/operating_point_005 | 0.33/0.33/0.33 | 0.5 | 400 | 208.5 | 2 |
| batch_dist_ternary_acetone+butan-1-ol+methanol/operating_point_006 | 0.33/0.33/0.33 | 0.33 | 700 | 308.5 | 1 |
| batch_dist_ternary_acetone+butan-1-ol+methanol/operating_point_007 | 0.33/0.33/0.33 | 4 | 600 | 140 | 1 |
| batch_dist_ternary_acetone+butan-1-ol+methanol/operating_point_008 | 0.33/0.33/0.33 | 2 | 500 | 592.5 | 2 |
| batch_dist_ternary_acetone+butan-1-ol+methanol/operating_point_009 | 0.33/0.33/0.33 | 3 | 450 | 240 | 1 |
| batch_dist_ternary_acetone+butan-1-ol+methanol/operating_point_010 | 0.33/0.33/0.33 | 4 | 500 | 308.5 | 0 |
| batch_dist_ternary_acetone+butan-1-ol+methanol/operating_point_011 | 0.33/0.33/0.33 | 0 | 500 | 309.5 | 1 |
| batch_dist_ternary_acetone+butan-1-ol+methanol/operating_point_012 | 0.33/0.33/0.33 | 2.5 | 500 | 208.5 | 4 |
| batch_dist_ternary_acetone+butan-1-ol+methanol/operating_point_013 | 0.33/0.33/0.33 | $\infty$ | 500 | 308.5 | 4 |
| batch_dist_ternary_butan-1-ol+propan-2-ol+water/operating_point_001 | 0.25/0.50/0.25 | 1 | 500 | 210 | 42 |
| batch_dist_ternary_butan-1-ol+propan-2-ol+water/operating_point_002 | 0.25/0.50/0.25 | 5 | 500 | 210 | 9 |
| batch_dist_ternary_butan-1-ol+propan-2-ol+water/operating_point_003 | 0.25/0.50/0.25 | 2.5 | 500 | 210 | 18 |
| batch_dist_ternary_butan-1-ol+propan-2-ol+water/operating_point_004 | 0.6/0.3/0.1 | 2.5 | 500 | 210 | 4 |
| batch_dist_ternary_butan-1-ol+propan-2-ol+water/operating_point_005 | 0.0025/0.0025/0.9950 | 2.5 | 500 | 210 | 1 |
| batch_dist_ternary_butan-1-ol+propan-2-ol+water/operating_point_006 | 0.05/0.05/0.90 | 2.5 | 500 | 210 | 1 |
| batch_dist_ternary_butan-1-ol+propan-2-ol+water/operating_point_007 | 0.25/0.5/0.25 | 5 | 200 | 210 | 1 |
| batch_dist_ternary_butan-1-ol+propan-2-ol+water/operating_point_008 | 0.25/0.5/0.25 | 1 | 200 | 210 | 4 |
| batch_dist_ternary_butan-1-ol+propan-2-ol+water/operating_point_009 | 0.25/0.5/0.25 | 1 | 450 | 210 | 7 |
| batch_dist_ternary_butan-1-ol+propan-2-ol+water/operating_point_010 | 0.25/0.5/0.25 | 1 | 600 | 210 | 1 |
| batch_dist_ternary_butan-1-ol+propan-2-ol+water/operating_point_011 | 0.25/0.5/0.25 | 2 | 600 | 210 | 3 |
| batch_dist_ternary_butan-1-ol+propan-2-ol+water/operating_point_012 | 0.25/0.5/0.25 | 5 | 750 | 210 | 10 |
| batch_dist_ternary_butan-1-ol+propan-2-ol+water/operating_point_013 | 0.25/0.5/0.25 | 1 | 600 | 280 | 2 |

**Table 5:** Continued.

| ID | Initial molar mixture composition | $R$ / - | $p$ / mbar | $\dot{Q}$ / W | No. of anomalies |
|---|---|---|---|---|---|
| batch_dist_ternary_butan-1-ol+propan-2-ol+water/operating_point_014 | 0.4/0.4/0.2 | 3 | 250 | 175 | 4 |
| batch_dist_ternary_butan-1-ol+propan-2-ol+water/operating_point_015 | 0.4/0.4/0.2 | 3 | 750 | 175 | 6 |
| batch_dist_ternary_butan-1-ol+propan-2-ol+water/operating_point_016 | 0.4/0.4/0.2 | 7.5 | 300 | 175 | 0 |
| batch_dist_ternary_butan-1-ol+propan-2-ol+water/operating_point_017 | 0.25/0.50/0.25 | 1 | 500 | 175 | 4 |
| batch_dist_ternary_butan-1-ol+propan-2-ol+water/operating_point_018 | 0.25/0.50/0.25 | 6 | 400 | 210 | 3 |
| batch_dist_ternary_butan-1-ol+propan-2-ol+water/operating_point_019 | 0.25/0.50/0.25 | 7.5 | 400 | 210 | 0 |
| batch_dist_ternary_butan-1-ol+propan-2-ol+water/operating_point_020 | 0.25/0.50/0.25 | 10 | 950 | 105 | 0 |
| batch_dist_ternary_butan-1-ol+propan-2-ol+water/operating_point_021 | 0.25/0.50/0.25 | 3 | 600 | 105 | 3 |
| batch_dist_ternary_butan-1-ol+propan-2-ol+water/operating_point_022 | 0.25/0.50/0.25 | 7.5 | 400 | 140 | 4 |
| batch_dist_ternary_butan-1-ol+propan-2-ol+water/operating_point_023 | 0.25/0.50/0.25 | 0.5 | 500 | 157.5 | 2 |
| batch_dist_ternary_butan-1-ol+propan-2-ol+water/operating_point_024 | 0.75/0.15/0.10 | 1 | 700 | 105 | 0 |
| batch_dist_ternary_butan-1-ol+propan-2-ol+water/operating_point_025 | 0.350/0.475/0.175 | 1 | 700 | 105 | 0 |
| batch_dist_ternary_butan-1-ol+propan-2-ol+water/operating_point_026 | 0.350/0.475/0.175 | 6 | 300 | 140 | 4 |
| batch_dist_ternary_butan-1-ol+propan-2-ol+water/operating_point_027 | 0.350/0.475/0.175 | 4 | 600 | 192.5 | 1 |
| batch_dist_ternary_butan-1-ol+propan-2-ol+water/operating_point_028 | 0.350/0.475/0.175 | 2 | 700 | 105 | 5 |
| batch_dist_ternary_butan-1-ol+propan-2-ol+water/operating_point_029 | 0.350/0.475/0.175 | 3 | 550 | 210 | 7 |
| batch_dist_ternary_butan-1-ol+propan-2-ol+water/operating_point_030 | 0.350/0.475/0.175 | 2 | 600 | 257.5 | 3 |
| batch_dist_ternary_butan-1-ol+propan-2-ol+water/operating_point_031 | 0.350/0.475/0.175 | 2 | 700 | 257.5 | 2 |
| batch_dist_ternary_butan-1-ol+propan-2-ol+water/operating_point_032 | 0.0025/0.0025/0.9950 | 2.5 | 500 | 208.5 | 1 |
| batch_dist_ternary_butan-1-ol+propan-2-ol+water/operating_point_033 | 0.05/0.05/0.9 | 2.5 | 500 | 208.5 | 0 |
| batch_dist_ternary_butan-1-ol+propan-2-ol+water/operating_point_034 | 0.25/0.50/0.25 | 0.5 | 500 | 210 | 0 |

# 4 Additional Process Data

In Figures 7-9, time-series data from additional sensors, as well as from relevant actuators, are shown for the examples described in the main manuscript.

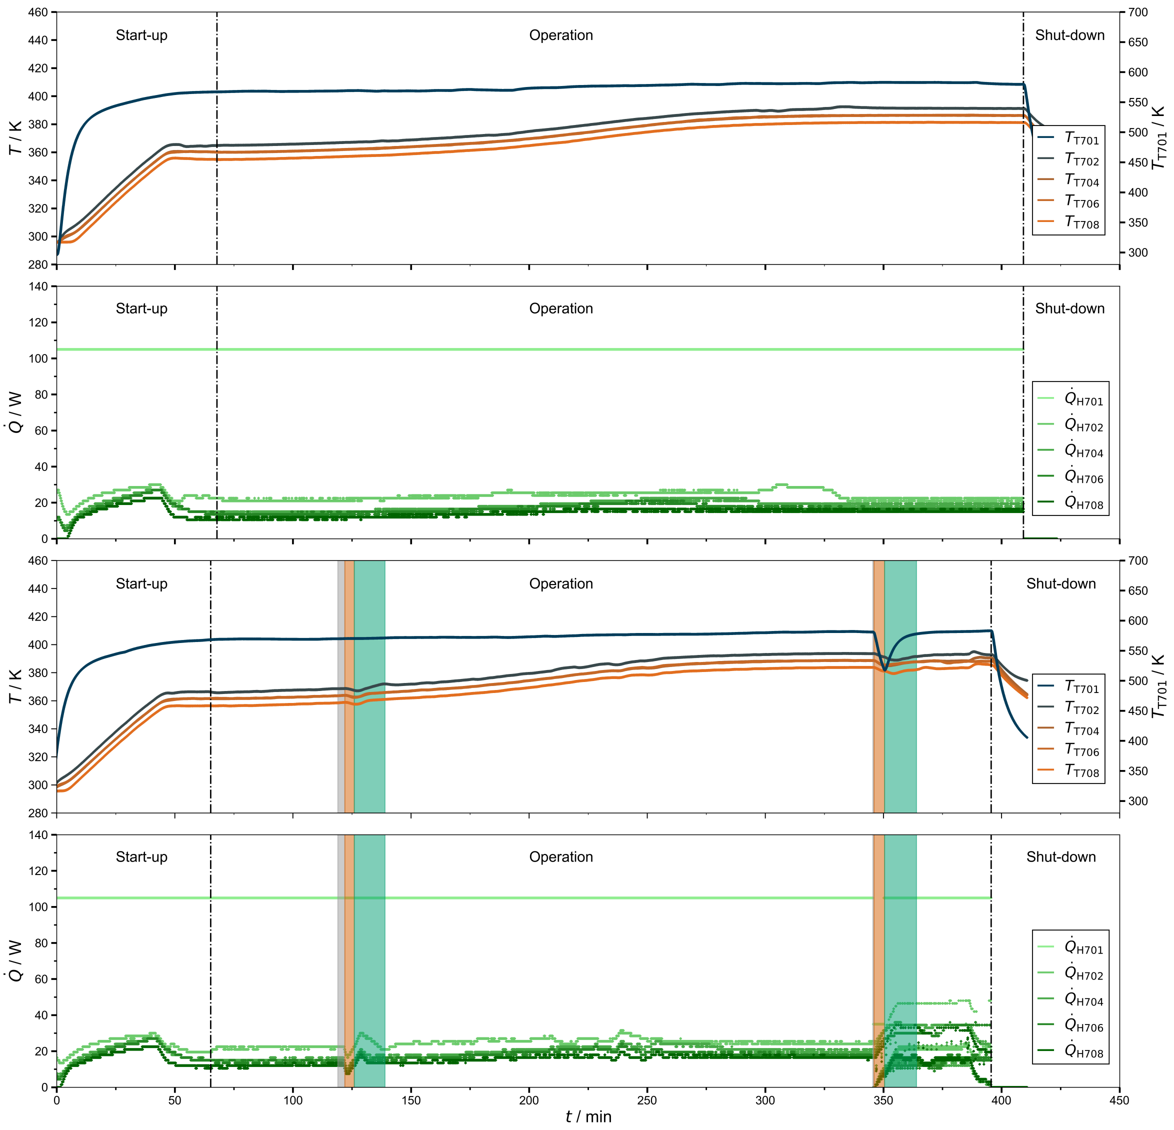


**Figure 7:** Two experiments carried out with the batch distillation plant. The upper two panels show results from a normal experiment (`batch_dist_ternary_butan-1-ol+propan-2-ol+water/operating_point_028/train_normal_experiment_001`), the lower two panels show the results from a corresponding anomalous experiment with two perturbations (`batch_dist_ternary_butan-1-ol+propan-2-ol+water/operating_point_028/test_anormal_experiment_001`). The colors indicate the three phases of the response to the perturbation. Both perturbations consist of changes of the setpoint of heating H002 in the reboiler vessel V001 (see text for details). In both experiments, batch distillation was performed at 700 mbar, a heat supply of 105 W, and a reflux ratio of 2.

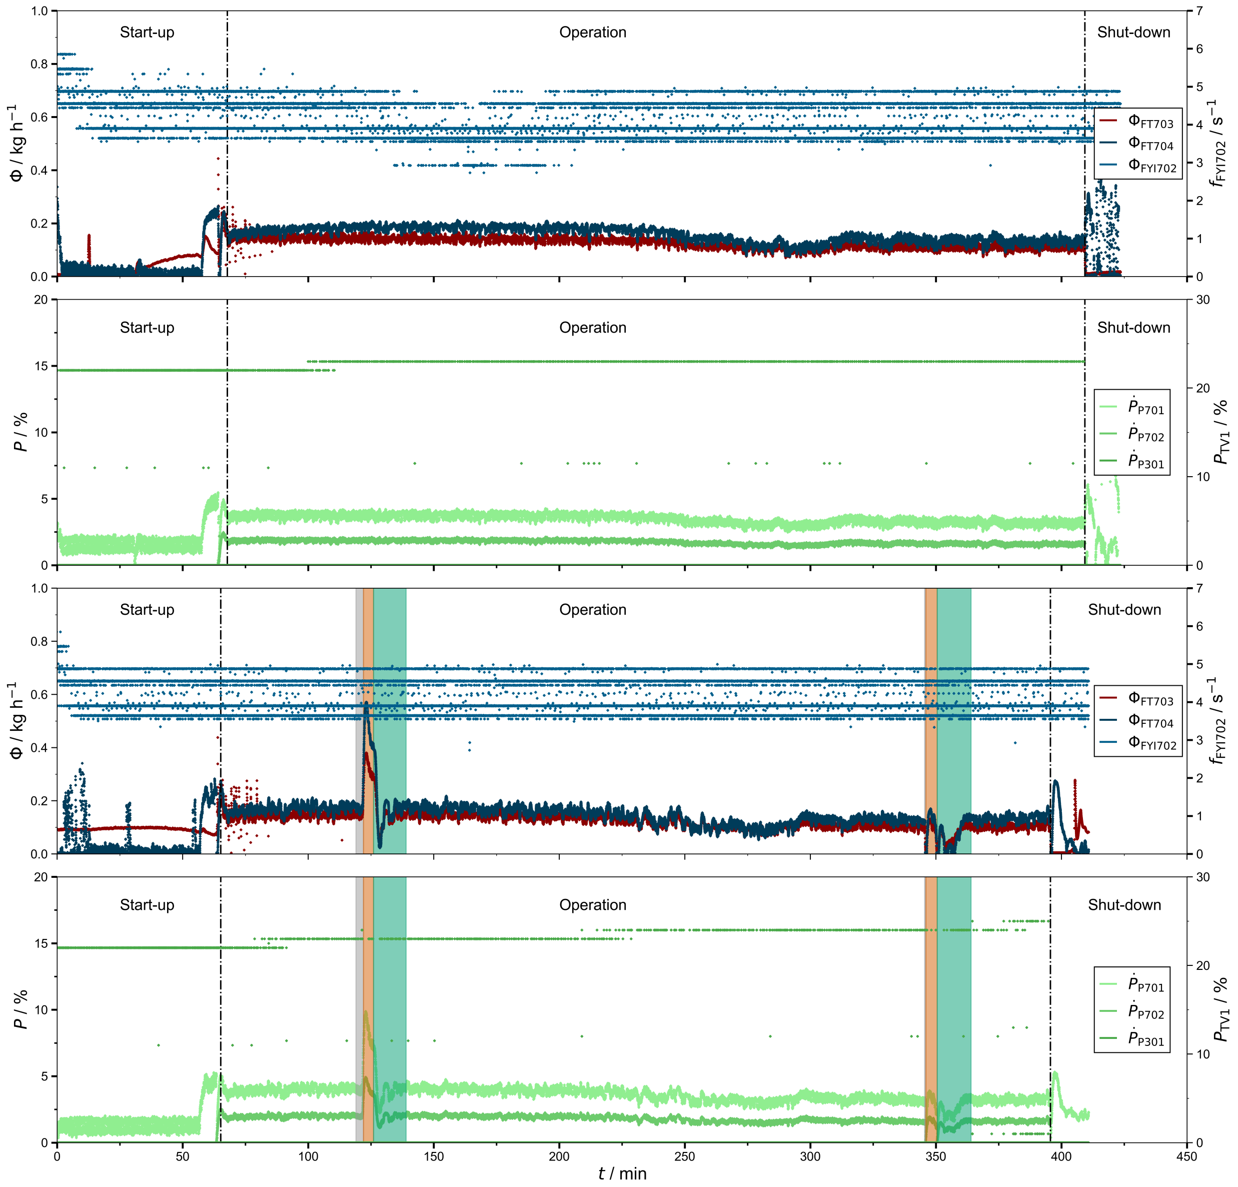


**Figure 8:** Two experiments carried out with the batch distillation plant. The upper two panels show results from a normal experiment (`batch_dist_ternary_butan-1-ol+propan-2-ol+water/operating_point_028/train_normal_experiment_001`), the lower two panels show the results from a corresponding anomalous experiment with two perturbations (`batch_dist_ternary_butan-1-ol+propan-2-ol+water/operating_point_028/test_anormal_experiment_001`). The colors indicate the three phases of the response to the perturbation. Both perturbations consist of changes of the setpoint of heating H002 in the reboiler vessel V001 (see text for details). In both experiments, batch distillation was performed at 700 mbar, a heat supply of 105 W, and a reflux ratio of 2.

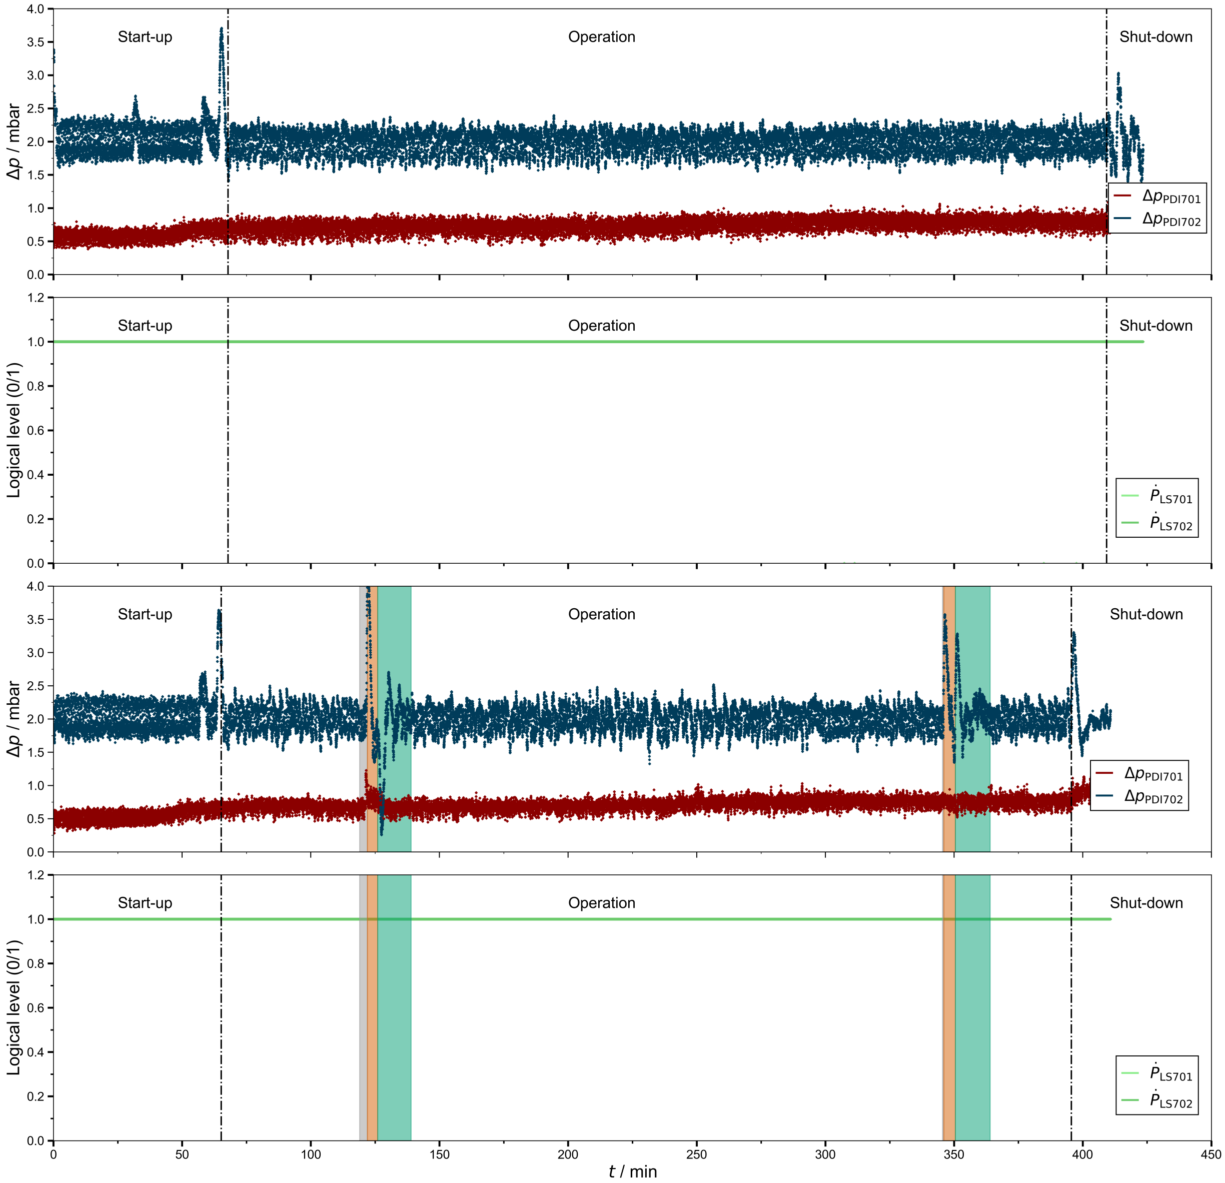


**Figure 9:** Two experiments carried out with the batch distillation plant. The upper two panels show results from a normal experiment (`batch_dist_ternary_butan-1-ol+propan-2-ol+water/operating_point_028/train_normal_experiment_001`), the lower two panels show the results from a corresponding anomalous experiment with two perturbations (`batch_dist_ternary_butan-1-ol+propan-2-ol+water/operating_point_028/test_anormal_experiment_001`). The colors indicate the three phases of the response to the perturbation. Both perturbations consist of changes of the setpoint of heating H002 in the reboiler vessel V001 (see text for details). In both experiments, batch distillation was performed at 700 mbar, a heat supply of 105 W, and a reflux ratio of 2.

# References


(1) Brombacher, W. G. *Mercury Barometers and Manometers*; U. S. Department of Commerce, National Bureau of Standards, 1960.

(2) Helmus, J. J.; Jaroniec, C. P. Nmrglue: an open source Python package for the analysis of multidimensional NMR data. *Journal of Biomolecular NMR* **2013**, *55*, 355–367.

(3) Cobas, C. Applications of the Whittaker smoother in NMR spectroscopy. *Magnetic Resonance in Chemistry* **2018**, *56*, 1140–1148.

(4) Zhang, F.; Tang, X.; Tong, A.; Wang, B.; Wang, J.; Lv, Y.; Tang, C.; Wang, J. Baseline correction for infrared spectra using adaptive smoothness parameter penalized least squares method. *Spectroscopy Letters* **2020**, *53*, 222–233.

(5) Erb, D. pybaselines: A Python library of algorithms for the baseline correction of experimental data. 2024.

(6) Li, D.-W.; Hansen, A. L.; Yuan, C.; Bruschweiler-Li, L.; Brüschweiler, R. DEEP picker is a deep neural network for accurate deconvolution of complex two-dimensional NMR spectra. *Nature Communications* **2021**, *12*.

(7) Friebel, A.; Specht, T.; von Harbou, E.; Münnemann, K.; Hasse, H. Prediction of flow effects in quantitative NMR measurements. *Journal of Magnetic Resonance* **2020**, *312*, 106683.

(8) Renon, H.; Prausnitz, J. M. Local Compositions in Thermodynamic Excess Functions for Liquid Mixtures. *AIChE Journal* **1968**, *14*, 135–144.

(9) Dortmund Data Bank. 2024; www.ddbst.com.
